# Supplementary material for: Cold pools, Breezes, and Monsoons: Propagating Convection over New Guinea
Source: arXiv:2506.00473 source file (2026-07-07)
Supplement: Supplementary file 1 [file SI-compress-250530.pdf]

# Supporting Information for "Cold pools, Breezes, and Monsoons: Propagating Convection over New Guinea"

Mingyue Tang<sup>1</sup>, Jimy Dudhia<sup>2</sup>, Changhai Liu<sup>2</sup>, Giuseppe Torri<sup>1</sup>

<sup>1</sup>Department of Atmospheric Sciences, University of Hawai'i at Mānoa, Honolulu, HI, USA

<sup>2</sup>National Center for Atmospheric Research, Boulder, CO, USA

## Contents of this file

1. Figures S1 to S6

## Introduction

This document contains additional text and figures that, while not critical, can facilitate the comprehension of the main manuscript.

In addition to this file, we have also uploaded two animations alongside the open-access resources on Zenodo:

1. Movie S1: Diurnal cycle of precipitation rate ( $\text{mm hr}^{-1}$ ) over New Guinea for all 12 months, based on 21-year averaged GPM data. (Movie1-12months-PRsnap.mp4)
2. Movie S2: ERA5 fields of relative humidity (RH), zonal wind (UU), and meridional wind (VV) around New Guinea for February 2010. (Movie2-Feb2010\_ERA5.mp4)

## Supplementary Figures

---

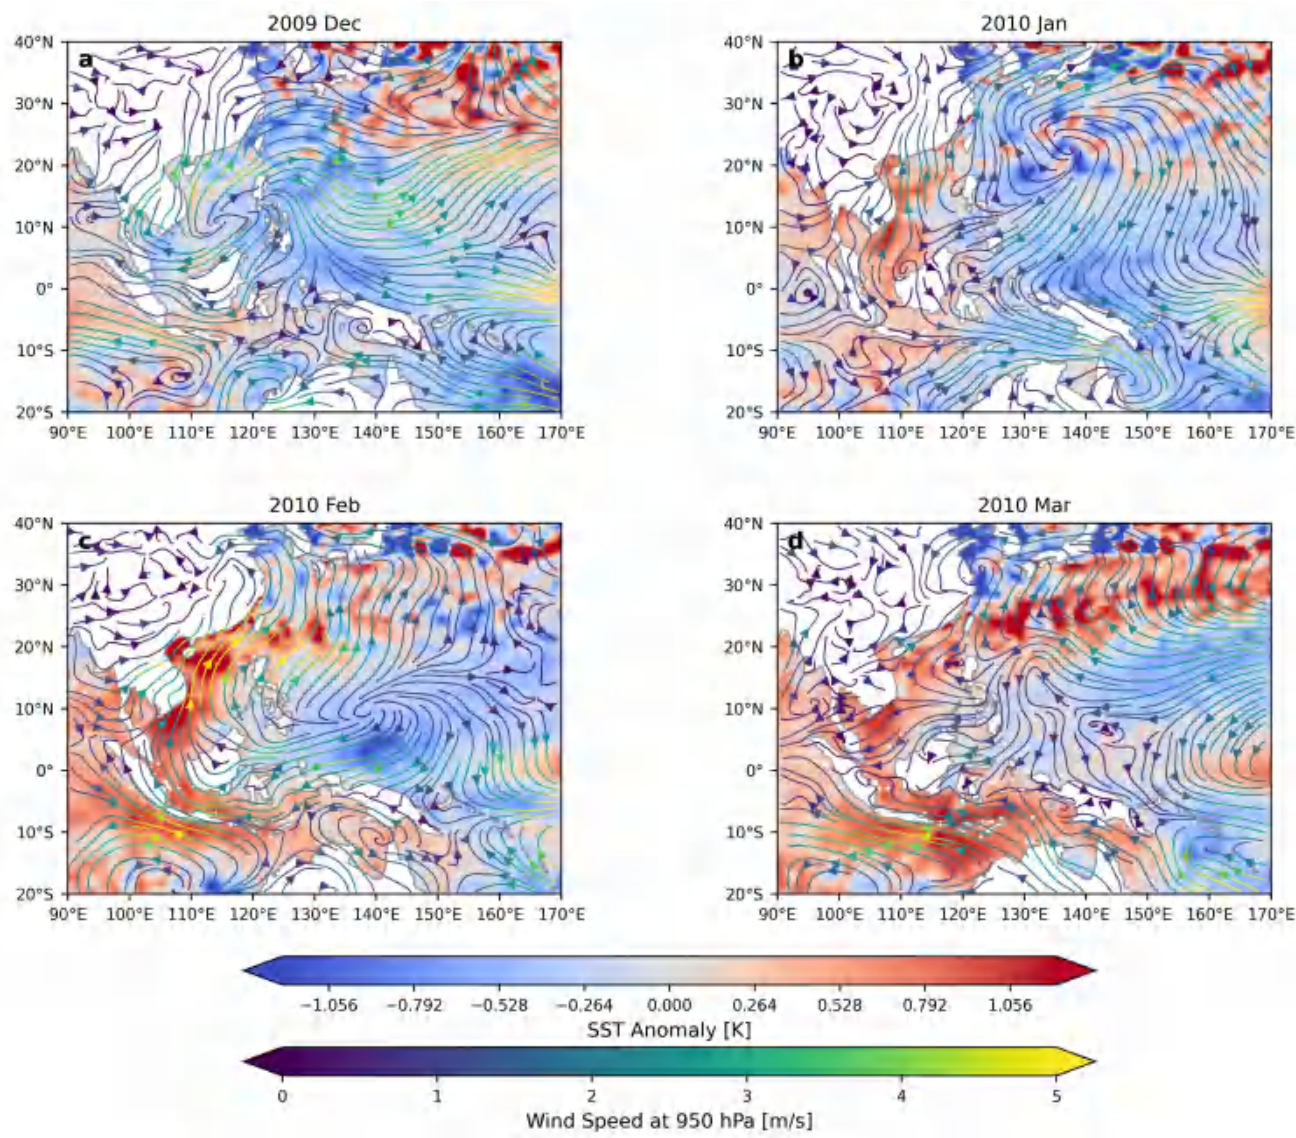

**Figure S1.** Monthly anomalies of SST (shading, in K) and 950 hPa wind streamlines (colored by wind speed in  $\text{m s}^{-1}$ ) from December 2009 to March 2010, based on 21-year ERA5 climatology. An evolving anti-cyclonic anomaly and SST cooling of approximately  $-0.5$  K appear northeast of New Guinea in February 2010 during the El Niño winter.

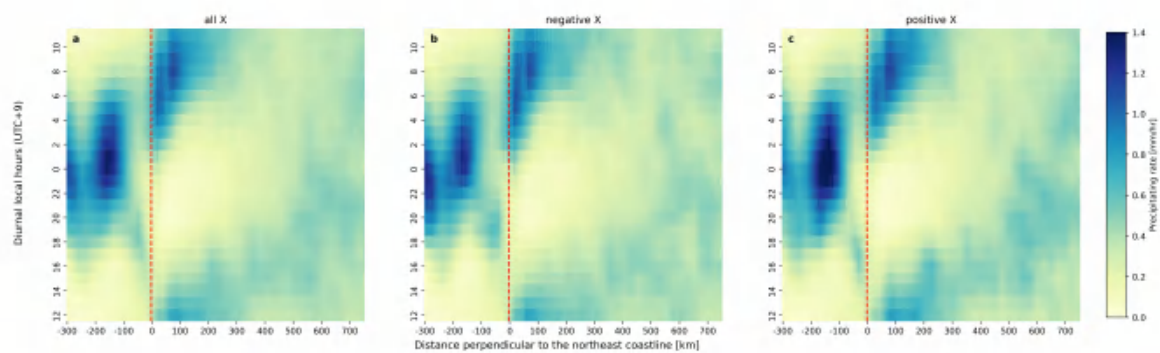

**Figure S2.** Same as Figure 3, but with the color scale capped at a maximum precipitation rate of  $1.4 \text{ mm hr}^{-1}$ .

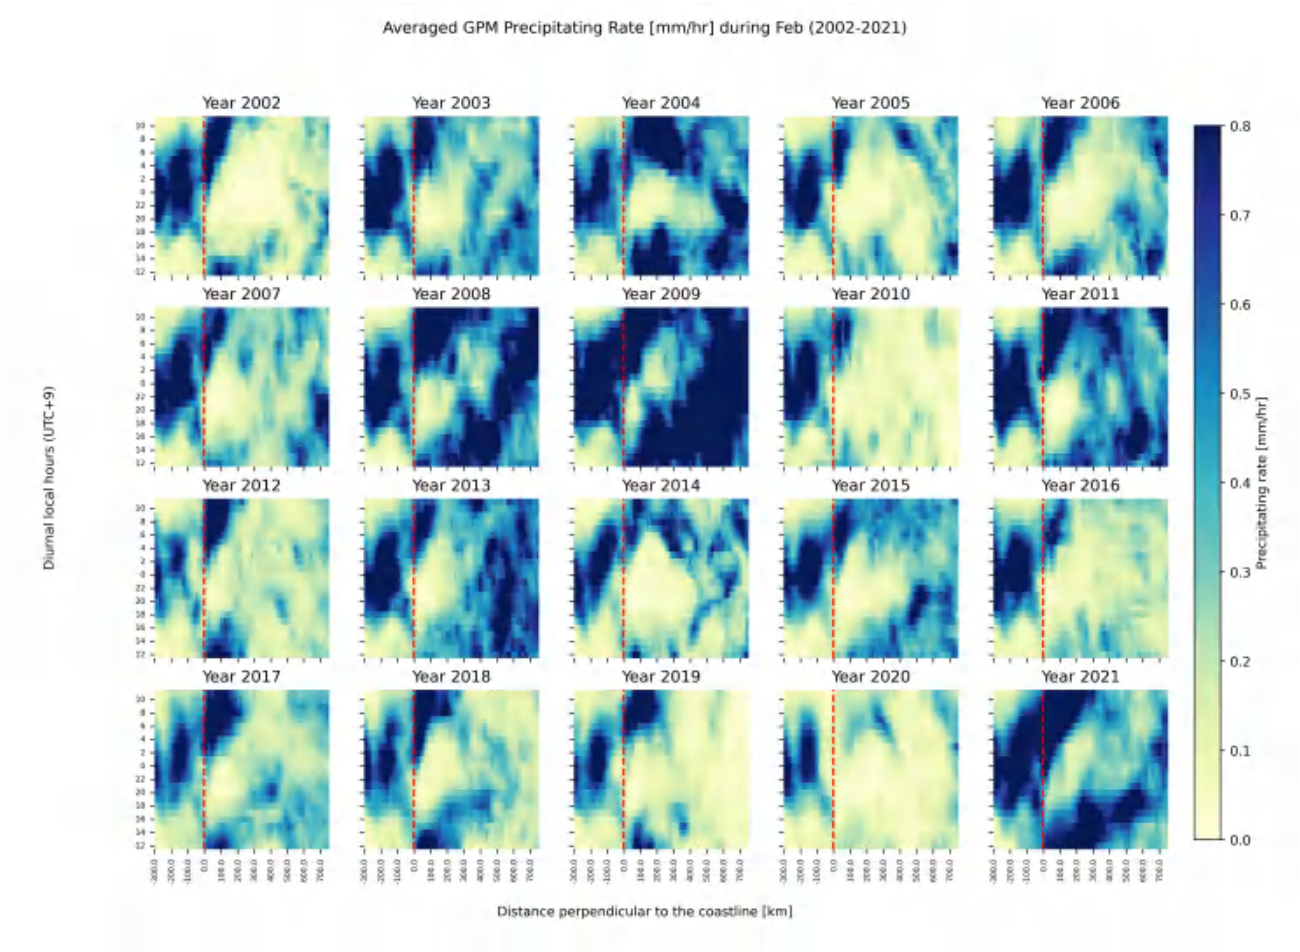

Figure S3. Same with Figure 3a, but separated 20 years from 2002-2021.

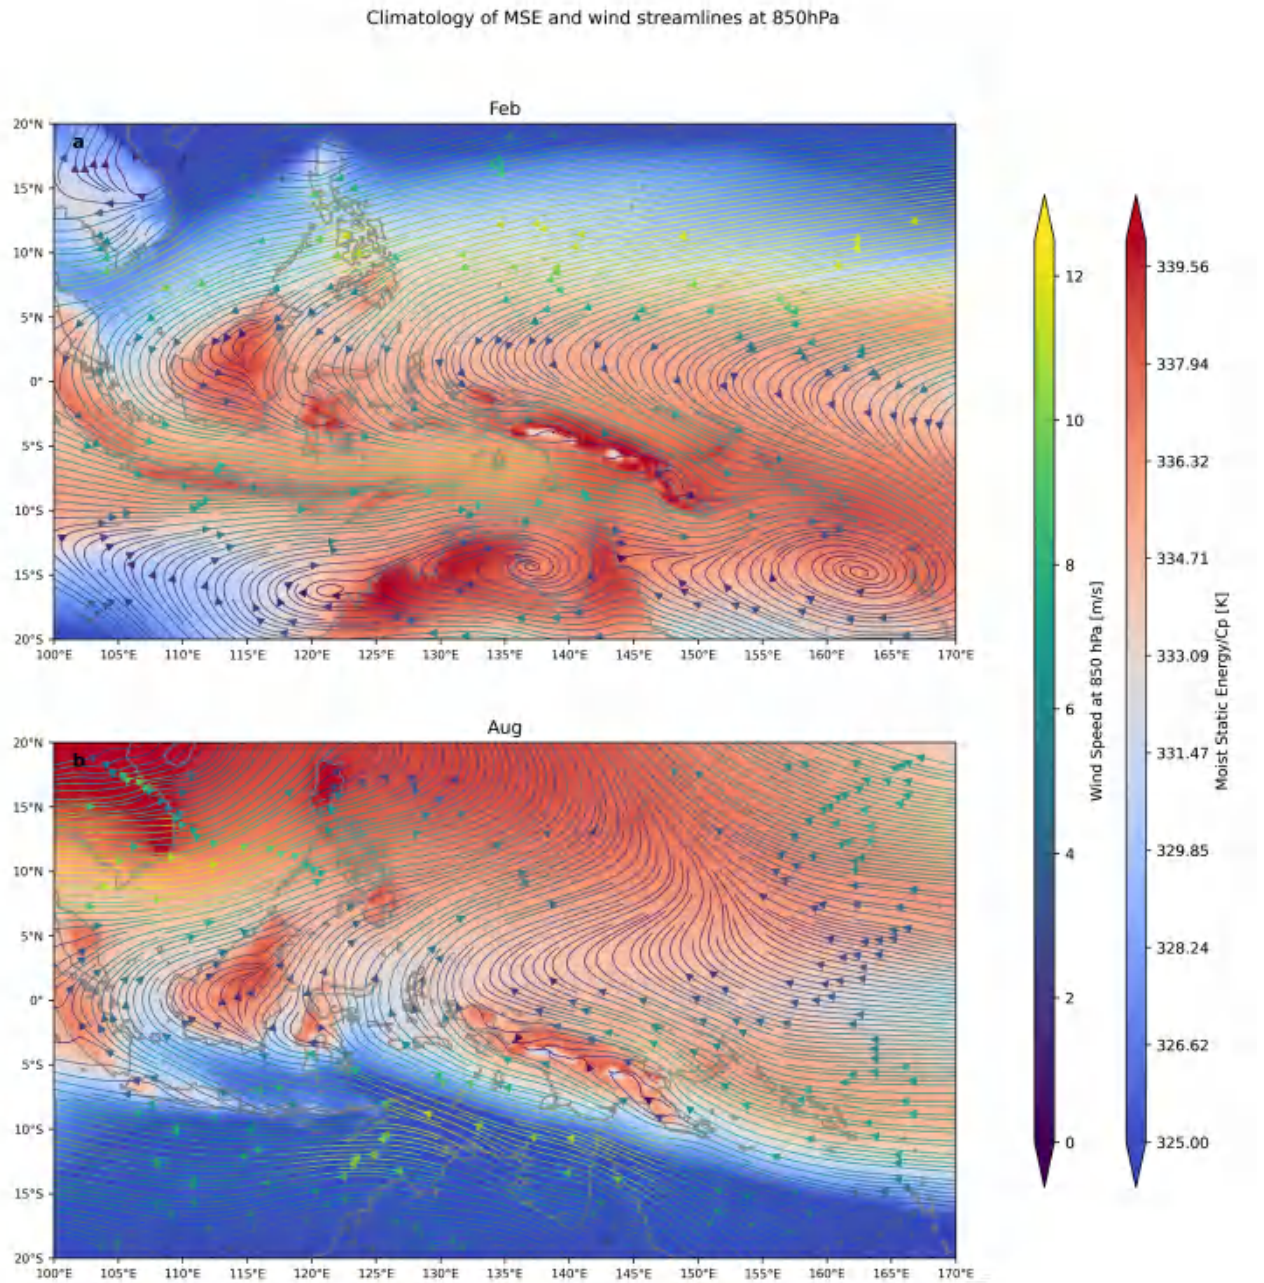

**Figure S4.** Climatological 850 hPa moist static energy normalized by  $C_p$  (shading, in K) and wind streamlines (colored by wind speed in  $\text{m s}^{-1}$ ) for February and August, based on 21-year ERA5 climatology.

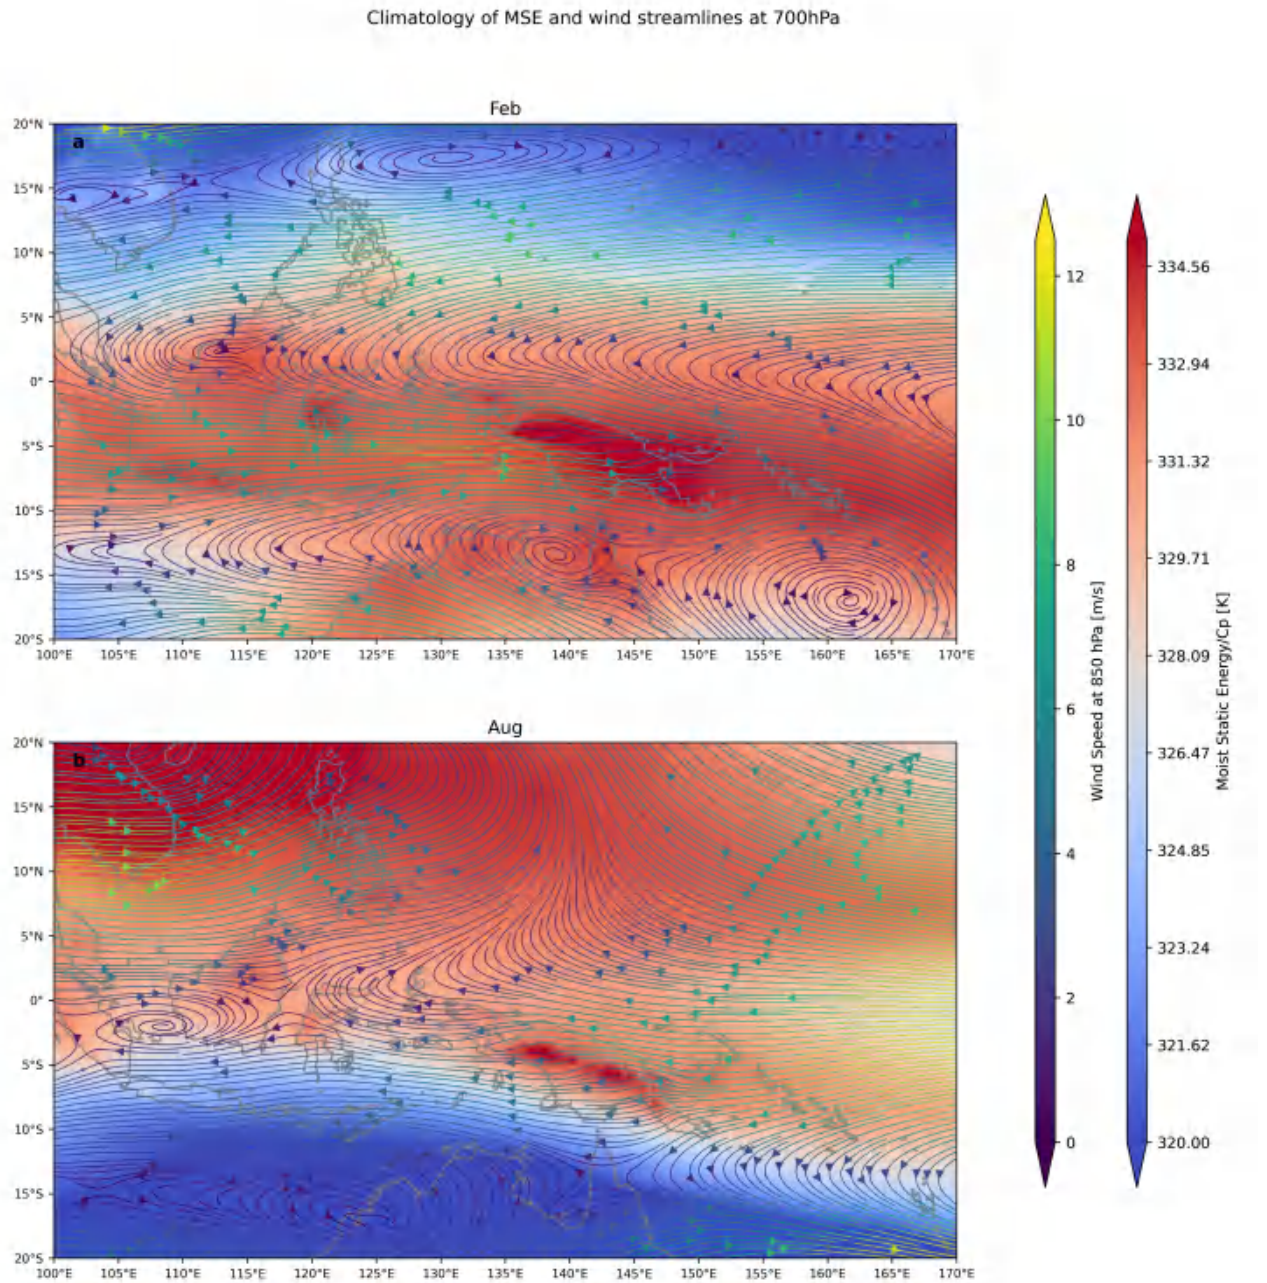

**Figure S5.** Climatological 700 hPa moist static energy normalized by  $C_p$  (shading, in K) and wind streamlines (colored by wind speed in  $\text{m s}^{-1}$ ) for February and August, based on 21-year ERA5 climatology.

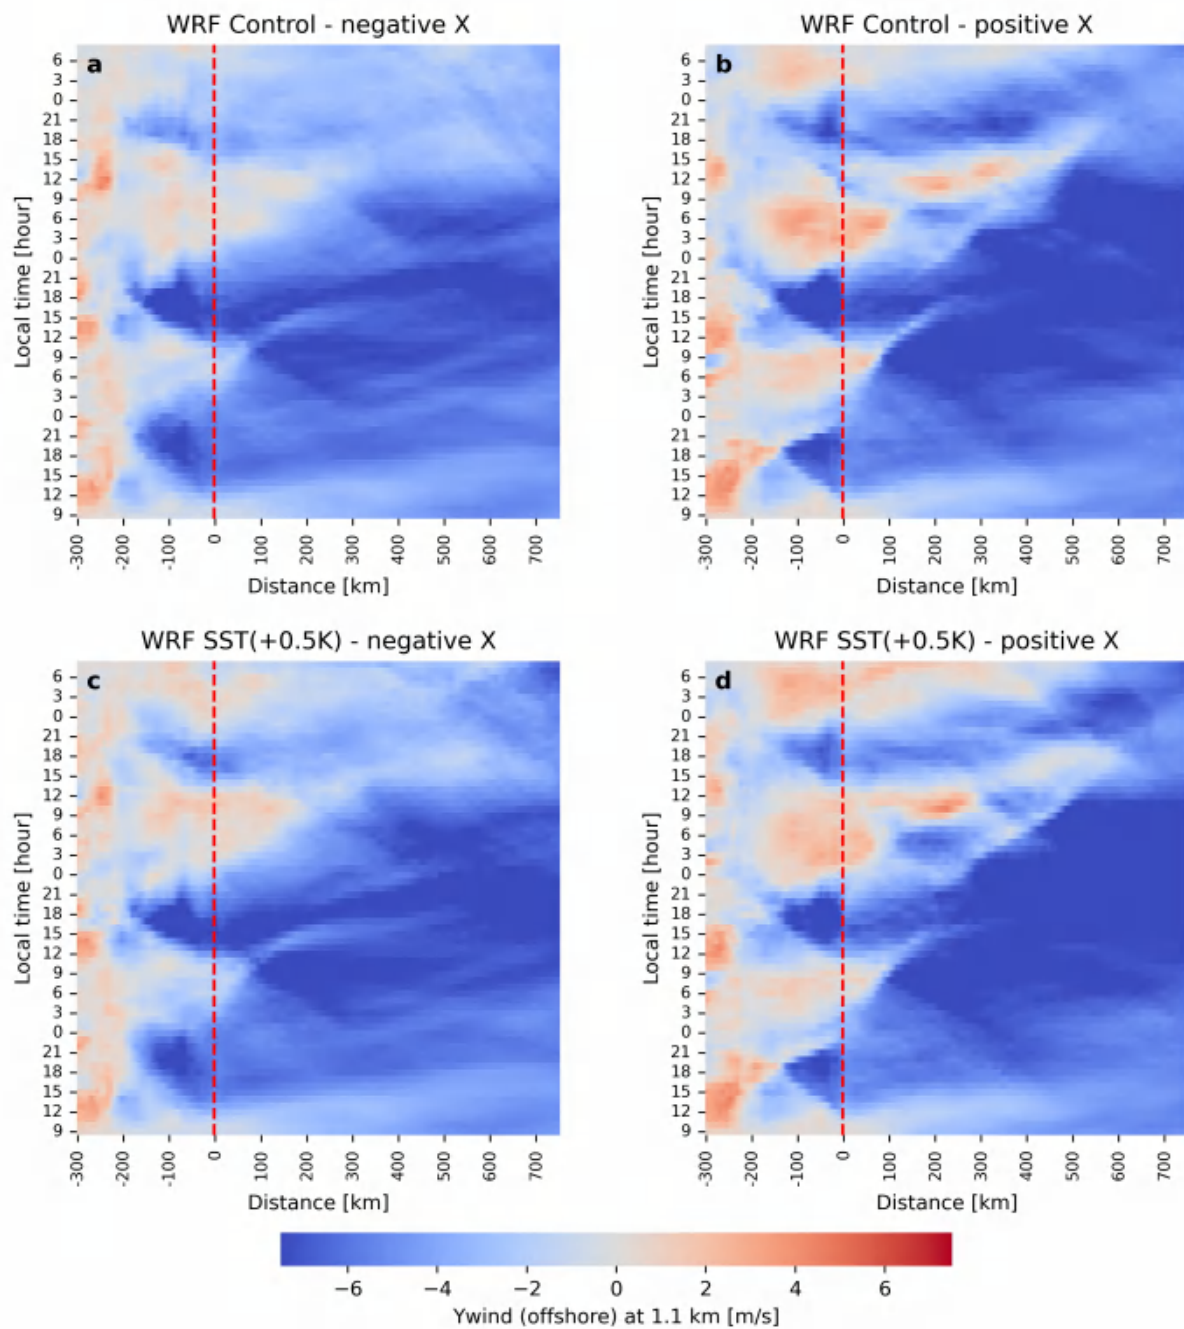

**Figure S6.** Same as Figure 7, but showing offshore wind speed ( $\text{m s}^{-1}$ ) at an altitude of 535 m.
